# Supplementary material for: Mathematical meal models for simulation of human metabolism
Source: arXiv:2307.16444 source file (2023-07-31)
Supplement: Supplementary file 1 [file linear_state_space_model_solution.tex]

\section{Solution to linear state space models}
% TOBK: JUST NOTES FOR MYSELF
% https://faculty.washington.edu/chx/teaching/me547/1-7_ss_sol.pdf
% https://math.stackexchange.com/questions/658276/integral-of-matrix-exponential

\begin{align}
    \dot x &= Ax + Bu
\end{align}

The solution is

\begin{align}
    x(t) &= e^{A(t - t_0)} x_0 + \int_{t_0}^t e^{A(t - \tau)} B u\, \mathrm d\tau
\end{align}

We assume $u$ to be constant and rearrange:

\begin{align}
    x(t) &= e^{A(t - t_0)} x_0 + e^{At} \int_{t_0}^t e^{-A\tau}\, \mathrm d\tau B u
\end{align}

If $A$ is non-singular,

\begin{align}
    \int_{t_0}^t e^{-A \tau} \mathrm d\tau = -(e^{-A t} - e^{-A t_0}) A^{-1}
\end{align}

if $A$ is singular, it can be written as

\begin{align}
    A &= U^{-1}
    \begin{bmatrix}
        A_{11} & 0 \\ 0 & A_{22}
    \end{bmatrix}
    U
\end{align}

where $A_{22}$ is non-singular and $A_{11}$ is strictly upper triangular. Then

\begin{align}
    e^{-At} = U^{-1}
    \begin{bmatrix}
        e^{-A_{11} t} & 0 \\ 0 & e^{-A_{22} t}
    \end{bmatrix}
    U
\end{align}

and

\begin{align}
    \int_{t_0}^t e^{-A\tau}
    &= U^{-1}
    \begin{bmatrix}
        \int_{t_0}^t e^{-A_{11} \tau} \mathrm d\tau & 0 \\ 0 & \int_{t_0}^t e^{-A_{22} \tau} \mathrm d\tau
    \end{bmatrix}
    U \nonumber \\
    &= U^{-1}
    \begin{bmatrix}
        \sum\limits_{k=0}^{K} \frac{(-1)^k}{k+1} \frac{(t^{k+1} - t_0^{k+1})}{k!} A_{11}^k & 0 \\ 0 & -(e^{-A_{22} t} - e^{-A_{22} t_0}) A_{22}^{-1}
    \end{bmatrix}
    U \nonumber \\
\end{align}

where $K$ is the largest number for which $A_{11}^K \neq 0$.
